# Supplementary material for: Generalizing Nonlinear ICA Beyond Structural Sparsity
Source: arXiv:2311.00866 source file (2023-11-01)
Supplement: Supplementary file 1 [file discuss_appendix.tex]

\section{Additional Discussion on Sparsity Assumptions} \label{sec:disc_ap}

Sparsity assumptions have been widely used in various fields. For latent variable models, sparsity in the generating process plays an important role in the disentanglement or identification of latent factors both empirically and theoretically \citep{bing2020adaptive, rohe2020vintage, moran2021identifiable, rhodes2021local, lachapelle2021disentanglement}. In causality, various versions of Occam's razor, such as faithfulness \citep{spirtes2000causation}, the minimality principle \citep{zhang2013comparison}, and frugality \citep{raskutti2018learning, forster2020frugal}, have been proposed to serve as fundamental assumptions for identifying the underlying causal structure.

Formulated as a measure of the density of dependencies, sparsity assumptions are more likely to be held when the observations are actually influenced by the sources in a ``simple” way. For example, in biology, analyses on ecological, gene-regulatory, metabolic, and other living systems find that active interactions may often be rather sparse \citep{busiello2017explorability}, even when these systems evolve with an unlimited number of complicated external stimuli. In physics, it is an important heuristic that a relatively small set of laws govern complicated observed phenomena. For instance, Einstein's theory of special relativity contains parsimonious relations between substances as an important heuristic to shave away the influence of ether compared to Lorentz's theory \citep{einstein1905does, nash1963nature}.

However, sparsity is not an irrefutable principle and our assumption may fail in a number of situations. The most direct one could be a scenario with heavily entangled relations between sources and observations. Let us consider the example of animal filmmaking in Sec. \ref{sec:ms}, where people are recording the sound of animals in a safari park. If the filming location is restricted to a narrow area of the safari park and multiple microphones are gathered together, the recording of each microphone will likely be influenced by almost all animals. In such a case, the dependencies between the recording of microphones and the animals are rather dense and our sparsity assumption is most likely not valid.

\looseness=-1
At the same time, even when the principle of simplicity holds, our formulation of sparsity, which is based on the sparse interactions between sources and observations, may still fail. One reason for this is the disparity between mechanism simplicity and structural sparsity. To illustrate this, one could consider the effect of sunlight on the shadow angles at the same location. In this case, the sun’s rays and the shadow angles act as the sources and the observations, respectively. Because rays of sunlight, loosely speaking, may be parallel to each other, the processes of them influencing the shadow angles may be almost identical. Thus, the influencing mechanism could be rather simple. On the other hand, each shadow angle is influenced by an unlimited number of the sun’s rays, which indicates that the interactions between them may not be sparse, therefore violating our assumption. This sheds light on one of the limitations of our sparsity assumption, because the principle of simplicity could be formulated in several ways. Besides, these different formulations also suggest various possibilities for identifiability based on simplicity assumptions. Another proposed assumption, i.e., independent influences, may be one of the alternative formulations, and more works remain to be explored in the future.
