# Supplementary material for: Generalizing Nonlinear ICA Beyond Structural Sparsity
Source: arXiv:2311.00866 source file (2023-11-01)
Supplement: Supplementary file 2 [file additional_discussion_appendix.tex]

\section{Additional Discussions}\label{sec:proofs}

\subsection{Assumptions for the identifiability with undercompleteness}
